# Supplementary material for: Spontaneous breaking of mirror symmetry beyond critical doping in Pb-Bi2212
Source: arXiv:2306.02621 source file (2023-09-08)
Supplement: Supplementary file 1 [file SHG_Supplementray_230513.pdf]

# Spontaneous breaking of mirror symmetry beyond critical doping in Pb-Bi2212 : Supplementary materials

Saegyeol Jung,<sup>1,2</sup> Byeongjun Seok,<sup>1,2</sup> Chang jae Roh,<sup>1,2</sup> Donghan Kim,<sup>1,2</sup> Yeonjae Lee,<sup>1,2</sup> San Kang,<sup>1,2</sup> Shigeyuki Ishida,<sup>3</sup> Shik Shin,<sup>4,\*</sup> Hiroshi Eisaki,<sup>3</sup> Tae Won Noh,<sup>1,2</sup> Dongjoon Song,<sup>1,5,†</sup> and Changyoung Kim<sup>1,2,‡</sup>

<sup>1</sup>Center for Correlated Electron Systems, Institute for Basic Science, Seoul, 08826, Korea

<sup>2</sup>Department of Physics and Astronomy, Seoul National University, Seoul, 08826, Korea

<sup>3</sup>National Institute of Advanced Industrial Science and Technology (AIST), Tsukuba, Ibaraki 305-8568, Japan

<sup>4</sup>Institute for Solid State Physics (ISSP), The University of Tokyo, Kashiwa, Chiba 277-8581, Japan

<sup>5</sup>Stewart Blusson Quantum Matter Institute, The University of British Columbia,  
2355 East Mall | Vancouver BC | V6T 1Z4 Canada

## 1. Temperature dependent resistivity behavior for dopings around $p_c$

As-grown Pb-Bi2212 crystals which have  $T_c = 79$  K with  $p \sim 0.205$  were annealed in  $N_2$  for 48 hours to control the doping level: (a) at  $700^\circ\text{C}$  for  $T_c = 93$  K and  $p \sim 0.175$  and (b) at  $550^\circ\text{C}$  for  $T_c = 85$  K and  $p \sim 0.195$ . The  $T_c$  is defined as the onset temperature of the Meissner effect and resistivity drop. Fig. S1 shows the doping and temperature dependent resistivity of Pb-Bi2212. The data exhibit typical temperature dependent behaviors of  $p < p_c$ ,  $p \sim p_c$  and  $p > p_c$ . In  $p < p_c$ , we can see a  $T$ -sublinear behavior ( $\rho \sim T^n, n < 1$ ), below the pseudogap temperature  $T^*$ . At  $p \sim p_c$ , the resistivity shows a  $T$ -linear behavior down to the superconducting temperature  $T_c$  while  $p > p_c$  exhibits a  $T$ -superlinear ( $\rho \sim T^n, n > 1$ ) behavior below  $T_{up}$ .

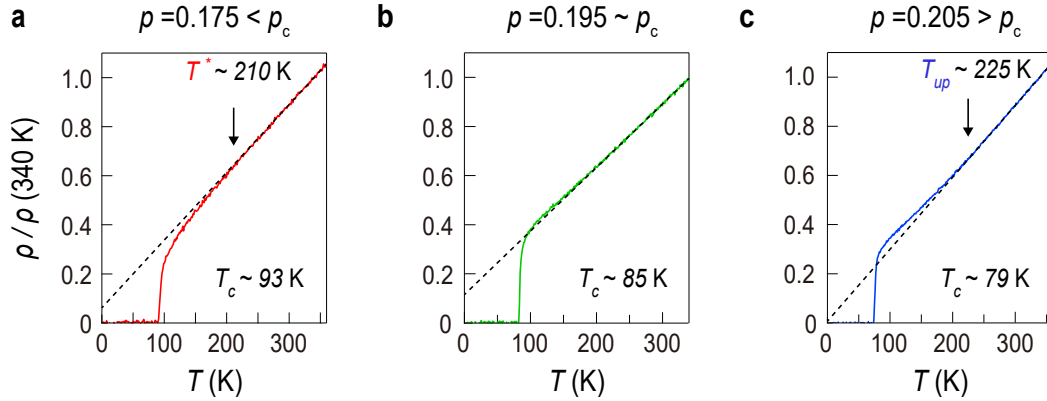

Fig. S1. **Temperature dependent normalized resistivity for Pb-Bi2212 for different doping regions.** (a-c) Temperature dependent resistivity curves for Pb-Bi2212 with  $p \sim 0.175$ ,  $0.195$  and  $0.205$  with  $p_c \sim 0.195$ . For  $p < p_c$  and  $p > p_c$ , the onset of the deviation from the linear resistivity is marked as  $T^*$  and  $T_{up}$ , respectively.

## 2. Mathematical expressions for SHG processes

Below, we list all of the mathematical expressions of the RA-SHG process which we consider in the main text. Effective polarization from electric dipole (ED), magnetic dipole (MD) and electric quadrupole (EQ) was calculated with the process  $P_i^{2\omega} \sim \chi_{ijk}^{ED} E_j E_k$ ,  $\nabla \times M \sim \nabla \times \chi_{ijk}^{MD} E_j E_k$  and  $\nabla \cdot Q \sim \nabla_j \chi_{ijkl}^{EQ} E_k E_l$ , respectively [1]. Here, we used the nomenclature employed in the work of Birss for each SHG process [2]. In the equations,  $\theta$  refers to the incidence angle of the incoming light relative to the (001) surface of the sample while  $\varphi$  is the angle of the incident plane about the  $c$ -axis, where  $\varphi = 0$  is taken to be the  $a$ -axis.

### ED

$\chi_{ijk}^{ED}$  tensor for 222 (D3) bulk electric dipole (non-centrosymmetric):

$$\left( \begin{array}{c|c|c} 0 & 0 & 0 \\ 0 & 0 & \chi_{xyz} \\ 0 & \chi_{xyz} & 0 \\ \hline 0 & 0 & \chi_{yxz} \\ 0 & 0 & 0 \\ \chi_{yxz} & 0 & 0 \\ \hline 0 & \chi_{zxy} & 0 \\ \chi_{zxy} & 0 & 0 \\ 0 & 0 & 0 \end{array} \right)$$

$$I_{PP}(2\omega) \sim |(\chi_{zxy} - \chi_{xyz} - \chi_{yxz})\cos^2(\theta)\sin(\theta)\sin(\varphi)\cos(\varphi)|^2$$

$$I_{SP}(2\omega) \sim |(\chi_{yxz}\cos^2(\varphi) - \chi_{xyz}\sin^2(\varphi))\sin(\theta)\cos(\theta)|^2$$

$$I_{PS}(2\omega) \sim |\chi_{zxy}\sin(\theta)\cos(\varphi)\sin(\varphi)|^2$$

$$I_{SS}(2\omega) \sim 0$$

$\chi_{ijk}^{ED}$  tensor for  $mm2$  (E3) bulk electric dipole (non-centrosymmetric):

$$\left( \begin{array}{c|c|c} 0 & 0 & \chi_{xxz} \\ 0 & 0 & 0 \\ \chi_{xxz} & 0 & 0 \\ \hline 0 & 0 & 0 \\ 0 & 0 & \chi_{yyz} \\ 0 & \chi_{yyz} & 0 \\ \hline \chi_{zxx} & 0 & 0 \\ 0 & \chi_{zyy} & 0 \\ 0 & 0 & \chi_{zzz} \end{array} \right)$$

$$I_{PP}(2\omega) \sim |\chi_{xxz}\sin^3(\theta) + \sin(\theta)\cos^2(\theta)((\chi_{zxx} - \chi_{xxz})\cos^2(\varphi) + (\chi_{zyy} - \chi_{yyz})\sin^2(\varphi))|^2$$

$$I_{SP}(2\omega) \sim |(\chi_{zxx}\sin^2(\varphi) + \chi_{zyy}\cos^2(\varphi))\sin^2(\theta)|^2$$

$$I_{PS}(2\omega) \sim |(\chi_{xxz} - \chi_{yyz})\cos(\theta)\sin(\theta)\sin(\varphi)\cos(\varphi)|^2$$

$$I_{SS}(2\omega) \sim 0$$

## MD

$\chi_{ijk}^{MD}$  tensor for 2/m (B3) bulk magnetic dipole (centrosymmetric):

$$\left( \begin{array}{c|c|c} 0 & 0 & \chi_{xxz} \\ 0 & 0 & \chi_{xyz} \\ \hline \chi_{xxx} & \chi_{xyz} & 0 \\ 0 & 0 & \chi_{yxz} \\ 0 & 0 & \chi_{yyz} \\ \hline \chi_{yxz} & \chi_{yyz} & 0 \\ \chi_{zxx} & \chi_{zxy} & 0 \\ \chi_{zxy} & \chi_{zyy} & 0 \\ 0 & 0 & \chi_{zzz} \end{array} \right)$$

$$I_{PP}(2\omega) \sim |\sin(\theta)\cos(\theta)((\chi_{xxz} - \chi_{yyz})\cos(\varphi)\sin(\varphi) - \chi_{yxz}\cos^2(\varphi) - \chi_{xyz}\sin^2(\varphi))|^2$$

$$I_{SP}(2\omega) \sim 0$$

$$I_{PS}(2\omega) \sim |\cos^2(\theta)\sin(\theta)((\chi_{zxx} - 2\chi_{xxz})\cos^2(\varphi) + (\chi_{zyy} - 2\chi_{yyz})\sin^2(\varphi) + \sin(\theta)\cos(\theta)(2\chi_{zxy} - 2\chi_{xyz} - 2\chi_{yxz}) + \chi_{zzz}\sin^3(\theta))|^2$$

$$I_{SS}(2\omega) \sim |\chi_{zxx}\sin(\theta)\sin^2(\varphi) + \chi_{zyy}\sin(\theta)\cos^2(\varphi) - 2\chi_{zxy}\sin(\theta)\cos(\varphi)\sin(\varphi)|^2$$

$\chi_{ijk}^{MD}$  tensor for  $mmm$  (D3) bulk magnetic dipole (centrosymmetric):

$$\left( \begin{array}{c|c|c} 0 & 0 & 0 \\ 0 & 0 & \chi_{xyz} \\ 0 & \chi_{xyz} & 0 \\ \hline 0 & 0 & \chi_{yxz} \\ 0 & 0 & 0 \\ \hline \chi_{yxz} & 0 & 0 \\ 0 & \chi_{zxy} & 0 \\ \chi_{zxy} & 0 & 0 \\ 0 & 0 & 0 \end{array} \right)$$

$$I_{PP}(2\omega) \sim |\sin(\theta)\cos(\theta)(\chi_{xyz}\sin^2(\varphi) - \chi_{yxz}\cos^2(\varphi))|^2$$

$$I_{SP}(2\omega) \sim 0$$

$$I_{PS}(2\omega) \sim |\cos^2(\theta)\sin(\theta)\sin(\theta)\cos(\theta)(\chi_{zxy} - \chi_{xyz} - \chi_{yxz})|^2$$

$$I_{SS}(2\omega) \sim |\chi_{zxy}\sin(\theta)\cos(\varphi)\sin(\varphi)|^2$$

$\chi_{ijk}^{MD}$  tensor for  $mm'm'$  (E3) bulk magnetic dipole (centrosymmetric):

$$\left( \begin{array}{c|c|c} 0 & 0 & \chi_{xxz} \\ 0 & 0 & 0 \\ \chi_{xxz} & 0 & 0 \\ \hline 0 & 0 & 0 \\ 0 & 0 & \chi_{yyz} \\ 0 & \chi_{yyz} & 0 \\ \hline \chi_{zxx} & 0 & 0 \\ 0 & \chi_{zyy} & 0 \\ 0 & 0 & \chi_{zzz} \end{array} \right)$$

$$I_{PP}(2\omega) \sim |\sin(\theta)\cos(\theta)(\chi_{xxz} - \chi_{yyz})\cos(\varphi)\sin(\varphi)|^2$$

$$I_{SP}(2\omega) \sim 0$$

$$I_{PS}(2\omega) \sim |\cos^2(\theta)\sin(\theta)((\chi_{zxx} - 2\chi_{xxz})\cos^2(\varphi) + (\chi_{zyy} - 2\chi_{yyz})\sin^2(\varphi) + \chi_{zzz}\sin^3(\theta))|^2$$

$$I_{SS}(2\omega) \sim |\chi_{zxx}\sin(\theta)\sin^2(\varphi) + \chi_{zyy}\sin(\theta)\cos^2(\varphi) - 2\chi_{zxy}\sin(\theta)\cos(\varphi)\sin(\varphi)|^2$$

## EQ

$\chi_{ijkk}^{EQ}$  tensor for 2/m (B4) bulk electric quadrupole (centrosymmetric):

$$\begin{pmatrix} \chi_{xxxx} & \chi_{xxxy} & 0 & \chi_{xyxx} & \chi_{xyxy} & 0 & 0 & 0 & \chi_{xzxz} \\ \chi_{xxyx} & \chi_{xxyy} & 0 & \chi_{xyyx} & \chi_{xyyy} & 0 & 0 & 0 & \chi_{xzyz} \\ 0 & 0 & \chi_{xxzz} & 0 & 0 & \chi_{xyzz} & \chi_{xzzx} & \chi_{xzzy} & 0 \\ \hline \chi_{yxxx} & \chi_{yxxy} & 0 & \chi_{yyxx} & \chi_{yyxy} & 0 & 0 & 0 & \chi_{yzxz} \\ \chi_{yxyx} & \chi_{yxyy} & 0 & \chi_{yyyx} & \chi_{yyyy} & 0 & 0 & 0 & \chi_{yzyz} \\ 0 & 0 & \chi_{yxzz} & 0 & 0 & \chi_{yyzz} & \chi_{yzzx} & \chi_{yzzy} & 0 \\ \hline 0 & 0 & \chi_{zxxz} & 0 & 0 & \chi_{zyxz} & \chi_{zzxx} & \chi_{zzxy} & 0 \\ 0 & 0 & \chi_{zxyz} & 0 & 0 & \chi_{zyyz} & \chi_{zzyx} & \chi_{zzyy} & 0 \\ \chi_{zxzx} & \chi_{zxzy} & 0 & \chi_{zyzx} & \chi_{zyzy} & 0 & 0 & 0 & \chi_{zzzz} \end{pmatrix}$$

$$\begin{aligned} I_{PP}(2\omega) \sim & |(-\chi_{yyyy})\sin^4(\varphi)\sin(\theta)\cos^3(\theta) + (\chi_{xyyy} + \chi_{yxyy} + \chi_{yyxy} + \chi_{yyyx})\sin^3(\varphi)\sin(\theta)\cos(\varphi)\cos^3(\theta) \\ & + (\chi_{zyyz} - \chi_{yyzz} + \chi_{zyzy})\sin^2(\varphi)\sin^3(\theta)\cos(\theta) + (-\chi_{xxyy} + \chi_{xyxy} + \chi_{xyyx} + \chi_{yxyx} \\ & + \chi_{yxyx} + \chi_{yyxx})\sin^2(\varphi)\sin(\theta)\cos^2(\varphi)\cos^3(\theta) + (\chi_{zzyy} - \chi_{yzzy} - \chi_{yzyz})\sin^2(\varphi)\sin(\theta)\cos^3(\theta) \\ & + ((\chi_{xyzz} + \chi_{yxzz}) - (\chi_{zxyz} + \chi_{zyxz}) - (\chi_{zzyy} + \chi_{zyyz}))\sin(\varphi)\sin^3(\theta)\cos(\varphi)\cos(\theta) + (2\chi_{xxyx} + \chi_{xyxx} \\ & + \chi_{yxxx})\sin(\varphi)\sin(\theta)\cos^3(\varphi)\cos^3(\theta) + ((\chi_{xzyz} + \chi_{yzxz}) + (\chi_{xzzz} + \chi_{yzzz}) \\ & - (\chi_{zzxy} + \chi_{zzyx}))\sin(\varphi)\sin(\theta)\cos(\varphi)\cos^3(\theta) + (\chi_{zxzx} - \chi_{xxzz} + \chi_{zxzx})\sin^3(\theta)\cos^2(\varphi)\cos(\theta) \\ & + \chi_{zzzz}\sin^3(\theta)\cos(\theta) + (-\chi_{xxxx})\sin(\theta)\cos^4(\varphi)\cos^3(\theta) + (\chi_{zzxx} - \chi_{xzzx} - \chi_{xzzx})\sin(\theta)\cos^2(\varphi)\cos^3(\theta)|^2 \end{aligned}$$

$$\begin{aligned} I_{SP}(2\omega) \sim & |(-\chi_{yyxx})/2)\sin^4(\varphi)\sin(2\theta) + (((\chi_{xyxx} + \chi_{yxxx} - \chi_{yyxy} - \chi_{yyyx}))/2)\sin^3(\varphi)\sin(2\theta)\cos(\varphi) \\ & + (((\chi_{xyxy} - \chi_{xxxx} + \chi_{xyyx} + \chi_{yxyx} + \chi_{yxyx} - \chi_{yyyy}))/2)\sin^2(\varphi)\sin(2\theta)\cos^2(\varphi) \\ & + ((\chi_{zzxx})/2)\sin^2(\varphi)\sin(2\theta) + (((\chi_{xyyy} - 2\chi_{xxyx} + \chi_{yxyy}))/2)\sin(\varphi)\sin(2\theta)\cos^3(\varphi) \\ & + (((\chi_{zzxy} + \chi_{zzyx}))/2)\sin(\varphi)\sin(2\theta)\cos(\varphi) + (-\chi_{xxyy})/2)\sin(2\theta)\cos^4(\varphi) \\ & + ((\chi_{zzyy})/2)\sin(2\theta)\cos^2(\varphi)|^2 \end{aligned}$$

$$\begin{aligned} I_{PS}(2\omega) \sim & |((\chi_{yyyy})/2)\sin^4(\varphi)\sin(2\theta)\cos(\theta) + (-((\chi_{xxyy} + \chi_{xyyx}))/2)\sin^3(\varphi)\sin(2\theta)\cos(\varphi)\cos(\theta) \\ & + \chi_{xyzz}\sin^2(\varphi)\sin^3(\theta) + \chi_{xzzz}\sin^2(\varphi)\sin(\theta)\cos^2(\theta) + (-((\chi_{xyxy}/2 \\ & - \chi_{yyyy}/2))/2)\sin^2(\varphi)\sin(2\varphi)\sin(2\theta)\cos(\theta) + (((\chi_{xxyx} - \chi_{yyxy}))/2)\sin^2(\varphi)\sin(2\theta)\cos^2(\varphi)\cos(\theta) \\ & + ((\chi_{xzyz})/2)\sin^2(\varphi)\sin(2\theta)\cos(\theta) + (((\chi_{xxyx}/2 + \chi_{yxyx}/2 - \chi_{yxyy}/2 \\ & - \chi_{yyyx}/2))/2)\sin(\varphi)\sin(2\varphi)\sin(2\theta)\cos(\varphi)\cos(\theta) + (((\chi_{yxyx} + \chi_{yyxx}))/2)\sin(\varphi)\sin(2\theta)\cos^3(\varphi)\cos(\theta) \\ & + (-((\chi_{xzzz}/2 - \chi_{yyzz}/2))\sin^3(\theta)\sin(2\varphi) + (-\chi_{yzzz})\sin^3(\theta)\cos^2(\varphi) + (-((\chi_{xzzx}/2 \\ & - \chi_{yzzz}/2))\sin(\theta)\sin(2\varphi)\cos^2(\theta) + (-\chi_{yzzx})\sin(\theta)\cos^2(\varphi)\cos^2(\theta) + (-((\chi_{xxxx}/2 \\ & - \chi_{yxyx}/2))/2)\sin(2\varphi)\sin(2\theta)\cos^2(\varphi)\cos(\theta) + (-((\chi_{xzzz}/2 - \chi_{yzyz}/2))/2)\sin(2\varphi)\sin(2\theta)\cos(\theta) \\ & + (-((\chi_{yxxx})/2)\sin(2\theta)\cos^4(\varphi)\cos(\theta) + (-\chi_{yzzz})/2)\sin(2\theta)\cos^2(\varphi)\cos(\theta)|^2 \end{aligned}$$

$$\begin{aligned} I_{SS}(2\omega) \sim & |\chi_{xyxx}\sin^4(\varphi)\sin(\theta) + (\chi_{xyxy} - \chi_{xxxx} + \chi_{yyxy} + \chi_{yyxx})\sin^3(\varphi)\sin(\theta)\cos(\varphi) \\ & + (\chi_{xyyy} - 2\chi_{xxyx} - \chi_{yxxx} + \chi_{yyxy} + \chi_{yyyx})\sin^2(\varphi)\sin(\theta)\cos^2(\varphi) + (-\chi_{xxyy} + \chi_{yxyx} + \chi_{yxyx} \\ & - \chi_{yyyy})\sin(\varphi)\sin(\theta)\cos^3(\varphi) + (-\chi_{yxyy})\sin(\theta)\cos^4(\varphi)|^2 \end{aligned}$$

$\chi_{ijkk}^{EQ}$  tensor for  $mmm$  (D4) bulk electric quadrupole (centrosymmetric):

$$\begin{pmatrix} \chi_{xxxx} & 0 & 0 & 0 & \chi_{xyxy} & 0 & 0 & 0 & \chi_{xzzx} \\ 0 & \chi_{xxyy} & 0 & \chi_{xyyx} & 0 & 0 & 0 & 0 & 0 \\ 0 & 0 & \chi_{xxzz} & 0 & 0 & 0 & \chi_{xzzx} & 0 & 0 \\ \hline 0 & \chi_{yxxy} & 0 & \chi_{yyxx} & 0 & 0 & 0 & 0 & 0 \\ \chi_{yxxy} & 0 & 0 & 0 & \chi_{yyyy} & 0 & 0 & 0 & \chi_{yzyz} \\ 0 & 0 & 0 & 0 & 0 & \chi_{yyzz} & 0 & \chi_{yzzz} & 0 \\ \hline 0 & 0 & \chi_{zxxx} & 0 & 0 & 0 & \chi_{zzxx} & 0 & 0 \\ 0 & 0 & 0 & 0 & 0 & \chi_{zyyz} & 0 & \chi_{zzyy} & 0 \\ \chi_{zxzx} & 0 & 0 & 0 & \chi_{zyzy} & 0 & 0 & 0 & \chi_{zzzz} \end{pmatrix}$$

$$\begin{aligned} I_{PP}(2\omega) \sim & |(-\chi_{yyyy})\sin^4(\varphi)\sin(\theta)\cos^3(\theta) + ((\chi_{xxzz} - \chi_{yyzz}) - (\chi_{zxzx} - \chi_{zyyz}) \\ & - (\chi_{zxxx} - \chi_{zyzy}))\sin^2(\varphi)\sin^3(\theta)\cos(\theta) + (-\chi_{xxyy} - \chi_{xxxx} + \chi_{xyxy} + \chi_{yyxx} + \chi_{yxyx} + \chi_{yxxy} \\ & + \chi_{yyxx}))\sin^2(\varphi)\sin(\theta)\cos^2(\varphi)\cos^3(\theta) + ((\chi_{xzzx} - \chi_{yzyz}) + (\chi_{xzzx} - \chi_{yzzz}) - (\chi_{zzxx} \\ & - \chi_{zzyy}))\sin^2(\varphi)\sin(\theta)\cos^3(\theta) + (\chi_{zxzx} - \chi_{xxzz} + (\chi_{zxzx} + \chi_{zzzz}))\sin^3(\theta)\cos(\theta) \\ & + (-\chi_{xxxx})\sin(\theta)\cos^2(\varphi)\cos^3(\theta) + (\chi_{zzxx} - \chi_{xzzx} - \chi_{xzzx})\sin(\theta)\cos^3(\theta)|^2 \end{aligned}$$

$$\begin{aligned} I_{SP}(2\omega) \sim & |(-\chi_{yyxx})\sin^4(\varphi)\sin(\theta)\cos(\theta) + (\chi_{zzxx} - \chi_{zzyy})\sin^2(\varphi)\sin(\theta)\cos(\theta) \\ & + (-\chi_{xxyy})\sin(\theta)\cos^4(\varphi)\cos(\theta) + (-\chi_{xyxy}/8 - \chi_{xxxx}/8 + \chi_{xyyx}/8 + \chi_{yxyx}/8 \\ & + \chi_{yxyx}/8 - \chi_{yyyy}/8))\sin(\theta)\cos(\theta)\cos(4\varphi) + (\chi_{zzyy} + (\chi_{xyxy}/8 - \chi_{xxxx}/8 + \\ & \chi_{xyyx}/8 + \chi_{yxyx}/8 + \chi_{yxyx}/8 - \chi_{yyyy}/8))\sin(\theta)\cos(\theta)|^2 \end{aligned}$$

$$\begin{aligned} I_{PS}(2\omega) \sim & |(-\chi_{xxyy} + \chi_{xyxy} + \chi_{yyxx} - \chi_{yyyy}))\sin^3(\varphi)\sin(\theta)\cos(\varphi)\cos^2(\theta) + (-\chi_{xxzz} \\ & - \chi_{yzyz}))\sin(\varphi)\sin^3(\theta)\cos(\varphi) + (\chi_{yxyx} - \chi_{xxxx} + \chi_{yxyx} + \chi_{yyxx})\sin(\varphi)\sin(\theta)\cos^3(\varphi)\cos^2(\theta) \\ & + (-\chi_{xzzx} - \chi_{yzyz}) - (\chi_{zzxx} - \chi_{yzzz}))\sin(\varphi)\sin(\theta)\cos(\varphi)\cos^2(\theta)|^2 \end{aligned}$$

$$\begin{aligned} I_{SS}(2\omega) \sim & |(\chi_{xyxy} - \chi_{xxxx} + \chi_{yxyx} + \chi_{yyxx})\sin^3(\varphi)\sin(\theta)\cos(\varphi) + (-\chi_{xxyy} + \chi_{yxyx} + \chi_{yxyx} \\ & - \chi_{yyyy}))\sin(\varphi)\sin(\theta)\cos^3(\varphi)|^2 \end{aligned}$$

$\chi_{ijkk}^{EQ}$  tensor for  $mm'm'$  (E4) bulk electric quadrupole (centrosymmetric):

$$\begin{pmatrix} 0 & \chi_{xxxy} & 0 & \chi_{xyxx} & 0 & 0 & 0 & 0 & 0 \\ \chi_{xxxy} & 0 & 0 & 0 & \chi_{xyyy} & 0 & 0 & 0 & \chi_{xzyz} \\ 0 & 0 & 0 & 0 & 0 & \chi_{xyzz} & 0 & \chi_{xzyz} & 0 \\ \hline \chi_{yxxx} & 0 & 0 & 0 & \chi_{yyxy} & 0 & 0 & 0 & \chi_{yzxz} \\ 0 & \chi_{yxyy} & 0 & \chi_{yyyx} & 0 & 0 & 0 & 0 & 0 \\ 0 & 0 & \chi_{yxzz} & 0 & 0 & 0 & \chi_{yzzx} & 0 & 0 \\ \hline 0 & 0 & 0 & 0 & 0 & \chi_{zyxz} & 0 & \chi_{zzxy} & 0 \\ 0 & 0 & \chi_{zxzy} & 0 & 0 & 0 & \chi_{zzyx} & 0 & 0 \\ 0 & \chi_{zxzy} & 0 & \chi_{zyzx} & 0 & 0 & 0 & 0 & 0 \end{pmatrix}$$

$$\begin{aligned} I_{PP}(2\omega) \sim & |(\chi_{yyyy} + \chi_{yyxy} + \chi_{yyxy} + \chi_{yyyx})\sin^3(\varphi)\sin(\theta)\cos(\varphi)\cos^3(\theta) + (-\chi_{zxyz} - \chi_{yxzz} - \chi_{xyzz} \\ & + \chi_{zxzy} + \chi_{zyxz} + \chi_{zyzx}))\sin(\varphi)\sin^3(\theta)\cos(\varphi)\cos(\theta) + (\chi_{xxxy} + \chi_{xxyx} + \chi_{xyxx} \\ & + \chi_{yxxx})\sin(\varphi)\sin(\theta)\cos^3(\varphi)\cos^3(\theta) + (\chi_{xzyz} + \chi_{xzzz} + \chi_{yzxz} + \chi_{yzzx} - \chi_{zzxy} \\ & - \chi_{zzyx})\sin(\varphi)\sin(\theta)\cos(\varphi)\cos^3(\theta)|^2 \end{aligned}$$

$$\begin{aligned} I_{SP}(2\omega) \sim & |(\chi_{xyxx} + \chi_{yxxx} - \chi_{yyxy} - \chi_{yyyx})\sin^3(\varphi)\sin(\theta)\cos(\varphi)\cos(\theta) \\ & + (-\chi_{xxxy} + \chi_{xxyx} - \chi_{xyyy} - \chi_{yxyy}))\sin(\varphi)\sin(\theta)\cos^3(\varphi)\cos(\theta) \\ & + (\chi_{zzxy} + \chi_{zzyx})\sin(\varphi)\sin(\theta)\cos(\varphi)\cos(\theta)|^2 \end{aligned}$$

$$\begin{aligned} I_{PS}(2\omega) \sim & |\chi_{yyyy}\sin^4(\varphi)\sin(\theta)\cos^2(\theta) + \chi_{xyzz}\sin^2(\varphi)\sin^3(\theta) + (\chi_{xxxy} + \chi_{xxyx} + \chi_{xyxx} - \chi_{yyxy} - \chi_{yyxy} \\ & - \chi_{yyyx})\sin^2(\varphi)\sin(\theta)\cos^2(\varphi)\cos^2(\theta) + (\chi_{xzyz} + \chi_{xzzz})\sin^2(\varphi)\sin(\theta)\cos^2(\theta) \\ & + (-\chi_{yxxx})\sin^3(\theta)\cos^2(\varphi) + (-\chi_{yxxx})\sin(\theta)\cos^4(\varphi)\cos^2(\theta) + (-\chi_{yzxz} - \chi_{yzzx})\sin(\theta)\cos^2(\varphi)\cos^2(\theta)|^2 \end{aligned}$$

$$\begin{aligned} I_{SS}(2\omega) \sim & |\chi_{xyxx}\sin^4(\varphi)\sin(\theta) + (\chi_{xyyy} - \chi_{xxyx} - \chi_{xxxy} - \chi_{yxxx} + \chi_{yxyy} \\ & + \chi_{yyxy} + \chi_{yyyx})\sin^2(\varphi)\sin(\theta)\cos^2(\varphi) + (-\chi_{yxyy})\sin(\theta)\cos^2(\varphi)|^2 \end{aligned}$$

### 3. Temperature dependent X-ray diffraction

To rule out the  $mmm$  to  $2/m$  bulk structural transition as the cause of the mirror symmetry breaking at  $T_{up}$ , we performed temperature dependent XRD for Pb-Bi2212. Data were obtained with D8 ADVANCE (Bruker) with  $Cu - K\alpha_1$  while the sample was aligned to the (001) axis. XRD data taken in the temperature range between 173 K ( $T < T_{up}$ ) and 297 K ( $T > T_{up}$ ) show no clear sign of a structural transition as shown in Fig. S2a. We plot zoom in view of the (0012) peak in Fig. S2b to show no signature of structural transition at  $T_{up}$ . Temperature evolution of the  $c$ -axis lattice parameter shows linear behavior from 173 K to 297 K (Fig. S2c). This linear temperature dependence of the lattice parameter may lead to the high temperature linear background in the temperature dependence of the SHG intensity.

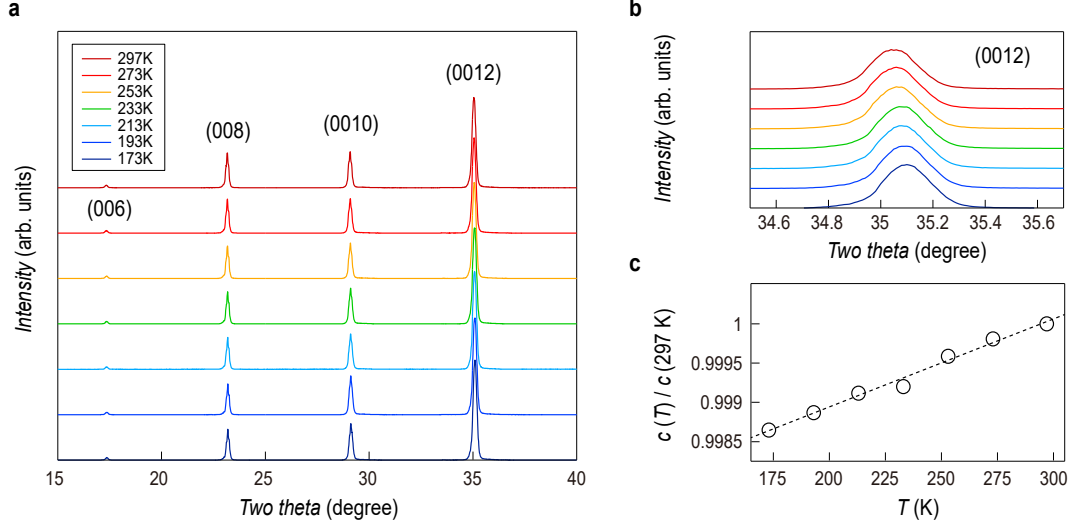

Fig. S2. **Temperature dependent X-ray diffraction data for Pb-Bi2212 ( $p=0.205$ ).** (a) Temperature dependent XRD for Pb-Bi2212 between 173 K ( $T < T_{up}$ ) and 297 K ( $T > T_{up}$ ). (b) Zoom in view of the (0012) peak. (c) Plot of the normalized  $c$ -axis lattice parameter as a function of temperature.

4. Temperature dependent RA-SHG intensity and integrated ARPES spectral weight difference without linear-in temperature background subtraction

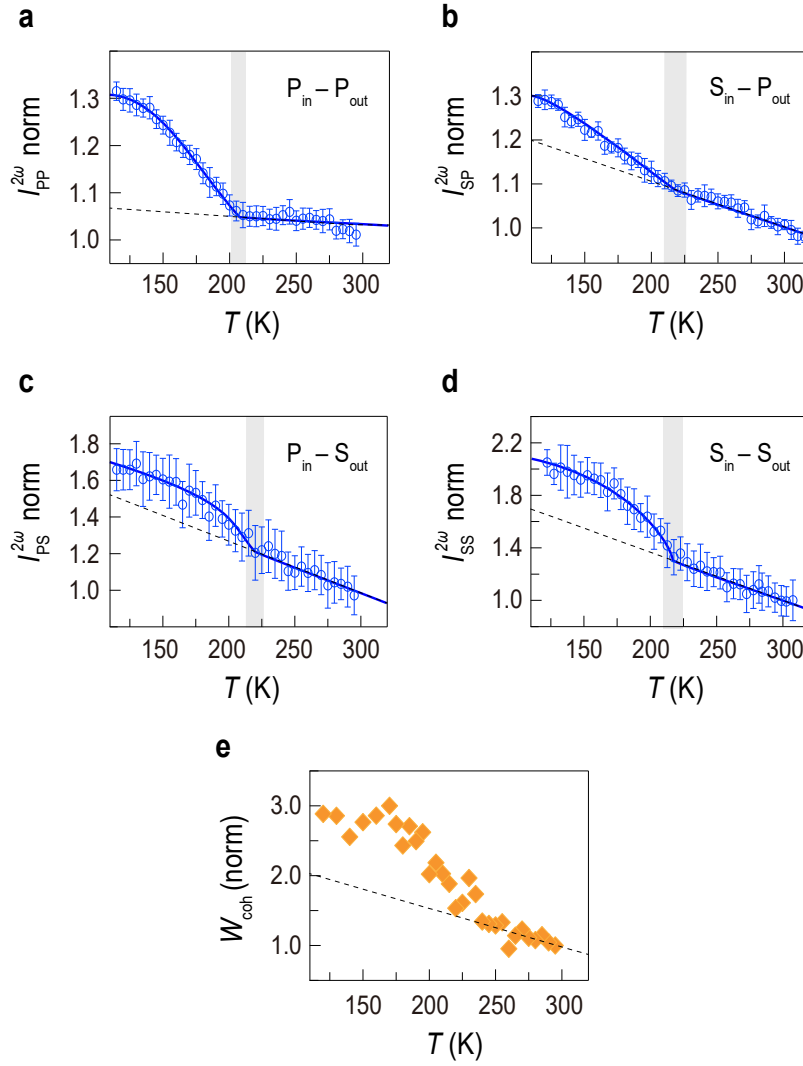

Fig. S3. (a-d) Temperature dependent SHG intensity used in Fig. 3. (e) Temperature dependence of the integrated ARPES spectral weight difference in Fig. 4f. Black dotted lines denote the subtracted linear background. Blue lines on the data are guides to the eyes. The width of the shaded grey interval shows the uncertainty in the transition temperature.

### 5. Fitting Pb-B212 RA-SHG results with EQ from $2/m$

As noted in the discussion section, we show the fitting results of the low temperature RA-SHG data in Figs. 2e-2h with the EQ contribution derived from the  $2/m$  point group. RA-SHG data in all polarization geometries (PP,SP,PS,SS) were fitted simultaneously with 28 non-zero independent tensor elements from  $2/m$  ( $\chi_{xxxx}, \chi_{xxxy}, \chi_{xxyy}, \chi_{xxzz}, \chi_{xyxx}, \chi_{xyyy}, \chi_{xyyz}, \chi_{xzzx}, \chi_{xzyz}, \chi_{yxxx}, \chi_{yxyx}, \chi_{yxyy}, \chi_{yxzz}, \chi_{yyxx}, \chi_{yyxy}, \chi_{yyzz}, \chi_{yzxx}, \chi_{yzzy}, \chi_{zxzx}, \chi_{zxzy}, \chi_{zyxz}, \chi_{zyzy}, \chi_{zzxx}, \chi_{zzxy}, \chi_{zzyy}, \chi_{zzzz}$ ).

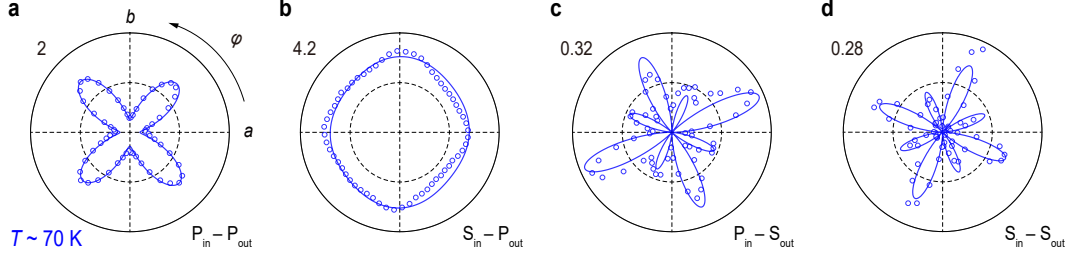

Fig. S4.  $2/m$  fitting result of RA-SHG data below  $T_{up}$ . RA-SHG data of Pb-Bi2212 collected under 4 polarization geometries: (a) PP, (b) SP, (c) PS, (d) SS at  $T \sim 70$  K ( $T < T_{up}$ ). All data sets are presented in the same intensity scale used in Fig. 2. RA-SHG data are fitted to the bulk EQ induced SHG from  $2/m$  (blue lines).

### 6. $mm'm'$ order parameter symmetry

Fig. S5 shows how low temperature PS channel data can be generated by a coherent superposition of  $\chi_{ijkl}^{EQ(i)}$  from  $mmm$  and  $\chi_{ijkl}^{EQ(c)}$  from  $mm'm'$ .

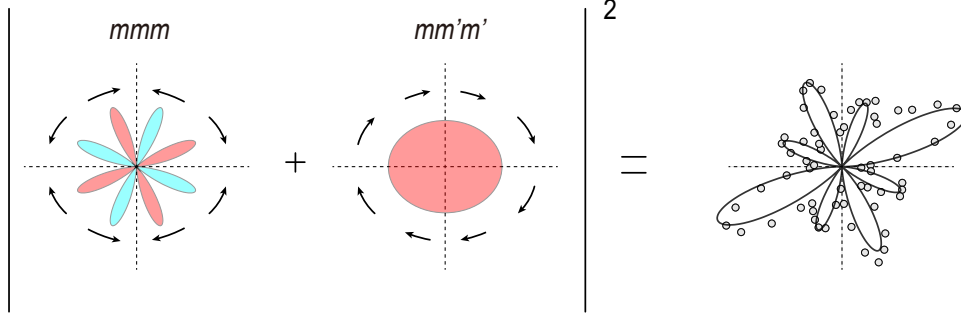

Fig. S5. **Construction of the PS channel data by a coherent superposition.** The schematic illustrates how the low temperature PS channel data can be reproduced by a coherent superposition of  $\chi_{ijkl}^{EQ(i)}$  from  $mmm$  and  $\chi_{ijkl}^{EQ(c)}$  from  $mm'm'$ . The black arrows indicate the induced polarization projected along the S-output direction. The black circle and line in the polar data denote RA-SHG data and the fitting result, respectively

### 7. Absence of surface reconstruction below $T_{up}$

To confirm the absence of surface reconstruction, we measured Fermi surfaces of Pb-Bi2212 below and above  $T_{up}$ . Figs. S6a and S6b show Fermi surface maps at  $T = 50$  K and 300 K, respectively. The Fermi surface maps were constructed by integrating the measured spectra over an energy window of  $E_F \pm 20$  meV. When there is a surface reconstruction, we expect to observe folded bands, that is, additional Fermi surfaces. In the data, we only see sharpening of the peaks without any additional Fermi surfaces across  $T_{up}$  (see Fig. S6c). For both temperatures, there is a superstructure band (S) between the main bands (M) which comes from significantly weakened but finite  $\text{BiO}_2$  modulation. This modulation breaks the C4 rotational symmetry of our sample, thus making the crystallographic point group of Pb-Bi2212 an  $mmm$ , not  $4/mmm$ .

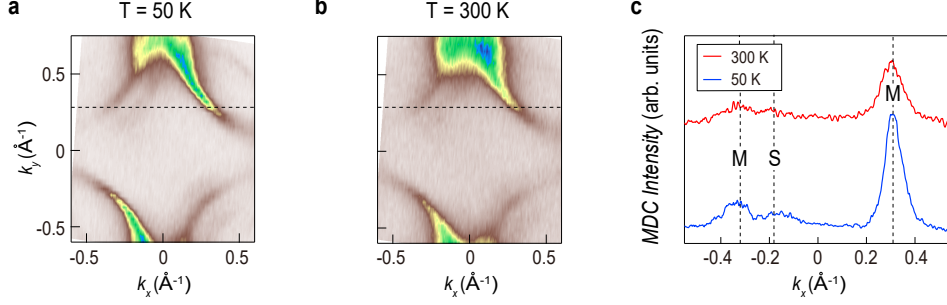

Fig. S6. **Pb-Bi2212 Fermi surface above and below  $T_{up}$ .** Fermi surfaces constructed by integrating over an energy window around the Fermi level ( $E_F \pm 20$  meV), taken at (a)  $T = 50$  K and (b) 300 K. (c) Temperature dependent momentum distribution curves (MDCs), integrated over  $0.28 \text{ \AA}^{-1} < k_y < 0.29 \text{ \AA}^{-1}$  around the black dotted lines in (a) and (b). M and S indicate the peaks from the main and superstructure bands, respectively.

### 8. On laser induced heating effect

In order to investigate the possible laser induced sample heating effect, we performed RA-SHG measurements in the SS geometry for two laser fluences of 2 and 3  $\text{mJ}/\text{cm}^2$  on different samples. We can see similar onset temperatures for the two laser fluences, which assures that our temperature dependent data obtained with 2  $\text{mJ}/\text{cm}^2$  is not significantly affected by laser heating.

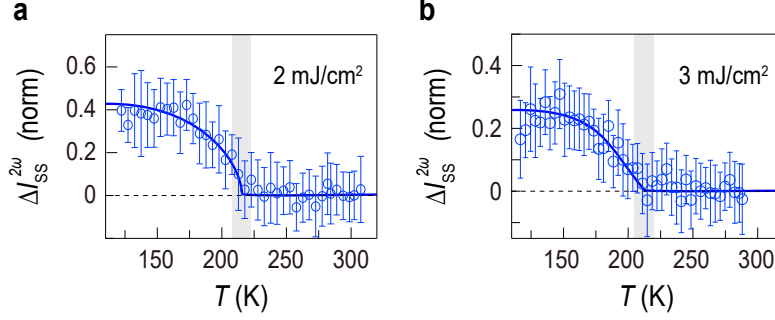

Fig. S7. **Fluence dependence in the temperature dependent RA-SHG intensity for SS geometry.** Temperature dependent RA-SHG intensity in the SS geometry for two laser fluences of (a) 2 and (b) 3  $\text{mJ}/\text{cm}^2$ . Data were first normalized to the values at  $T \sim 295$  K. Then, a high-temperature linear background was subtracted from each data. The error bars denote the standard deviation of 60 measurements taken within a 5 K temperature window while increasing the temperature at a ramping rate of 2 K/min.

### 9. GaAs(110) RA-SHG data for the alignment

Before each RA-SHG experiment, we measured two references for the system alignment: (1) gold mirror and (2) GaAs (110). With the gold mirror, we monitor the isotropy of the SHG intensity to check if the incident angle remains the same while rotating the incident plane over the full polar angle  $\varphi$  [3]. Then, we used GaAs(110) sample to make input and output polarizers parallel to each other. Room temperature RA-SHG data from GaAs(110) are fitted to bulk electric dipole induced SHG from  $\bar{4}3m$  (red lines in Fig.S8). Equal intensities of adjacent lobes ( $I_A$  and  $I_B$ ) in the SP channel data indicate parallelity of input and output polarizers. We note that the fitting function for bulk electric dipole induced SHG from  $\bar{4}3m$  is unable to fit the PS channel data. This suggests the additional surface contribution to the SHG [4]. However, we will not discuss the exact surface point group in the detail.

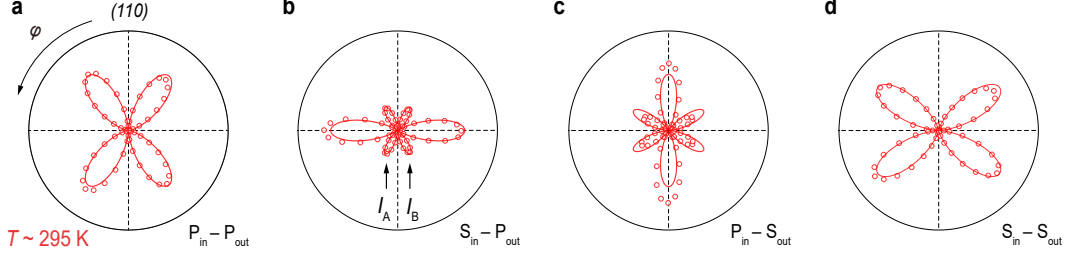

Fig. S8. **RA-SHG data from GaAs(110) collected under 4 polarization geometries.** (a) PP, (b) SP, (c) PS, and (d) SS at  $T \sim 295$  K. The room temperature data are fitted to bulk electric dipole induced SHG from  $\bar{4}3m$  (red lines).

### 10. Position dependence of the mirror symmetry breaking order

To check if the observed mirror symmetry breaking order has any position dependence on the sample, we scanned the sample in  $10\ \mu\text{m}$  steps while monitoring the intensity difference between adjacent lobes ( $I_A$  and  $I_B$  in Fig. S8b) along the mirror plane (Figs. S9a and S9b). Compared to the nearly identical intensities for the two adjacent lobes at room temperature, we observe a significant intensity difference between the two lobes ((Fig. S9b). Moreover, the normalized intensity difference is more or less position independent as shown in Fig. S9c.

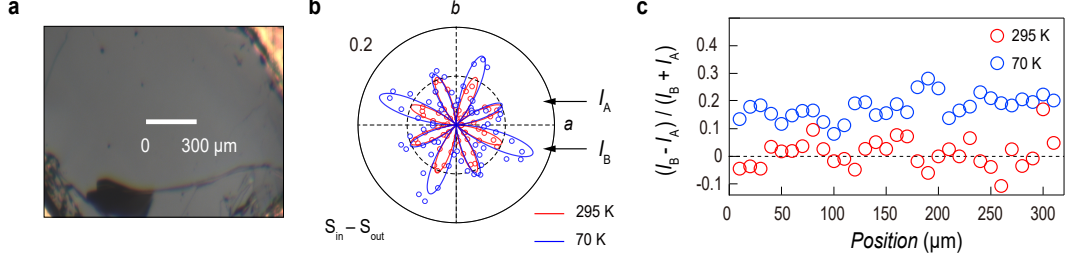

Fig. S9. **Position dependence on the signature of mirror symmetry breaking.** (a) Optical microscope image of a cleaved Pb-Bi2212 surface. The white line marks the scan range for the position dependence measurement. (b) RA-SHG polar pattern in the SS geometry at  $T = 295\text{ K}$  and  $70\text{ K}$ . The  $295\text{ K}$  data was fitted to EQ induced SHG from  $mmm$  (red line) while the  $70\text{ K}$  data was fitted to the coherent superposition of EQ induced SHG from  $mmm$  and  $mm'm'$  (blue line). (c) Position dependence of the normalized intensity difference  $(I_B - I_A) / (I_B + I_A)$  for the two adjacent lobes along the mirror plane, measured with  $10\ \mu\text{m}$  steps. SHG intensity at each position was measured for 10 s.

### 11. Doping dependent electronic structures below and above $p_c$

Figure S10 shows doping and temperature dependent electronic structure of Pb-Bi2212 for  $p = 0.195 < p_c$  and  $p = 0.205 > p_c$ . All the data were divided by the energy resolution convolved Fermi-Dirac function. It was recently reported that the antinodal energy distribution curve (EDC) abruptly broadens and becomes incoherent below the critical doping  $p_c$  [5]. Therefore, one can determine whether the doping is below or above  $p_c$  by investigating the EDC at the antinode (red dotted line in panels (a) and (b)) at 280 K. We see that the spectra taken at 280 K in Fig. S10d shows a quasiparticle-like peak near the Fermi level, a phenomenological character for  $p > p_c$ , in contrast to the data for  $p < p_c$  in Fig. S10c which display a broad incoherent behavior. We also noted that the coherent bilayer splitting between the bonding and anti-bonding states appears below  $T_{up}=225$  K as described in the main text. This consistency further shows that the doping level of our sample is beyond the critical doping  $p_c$ .

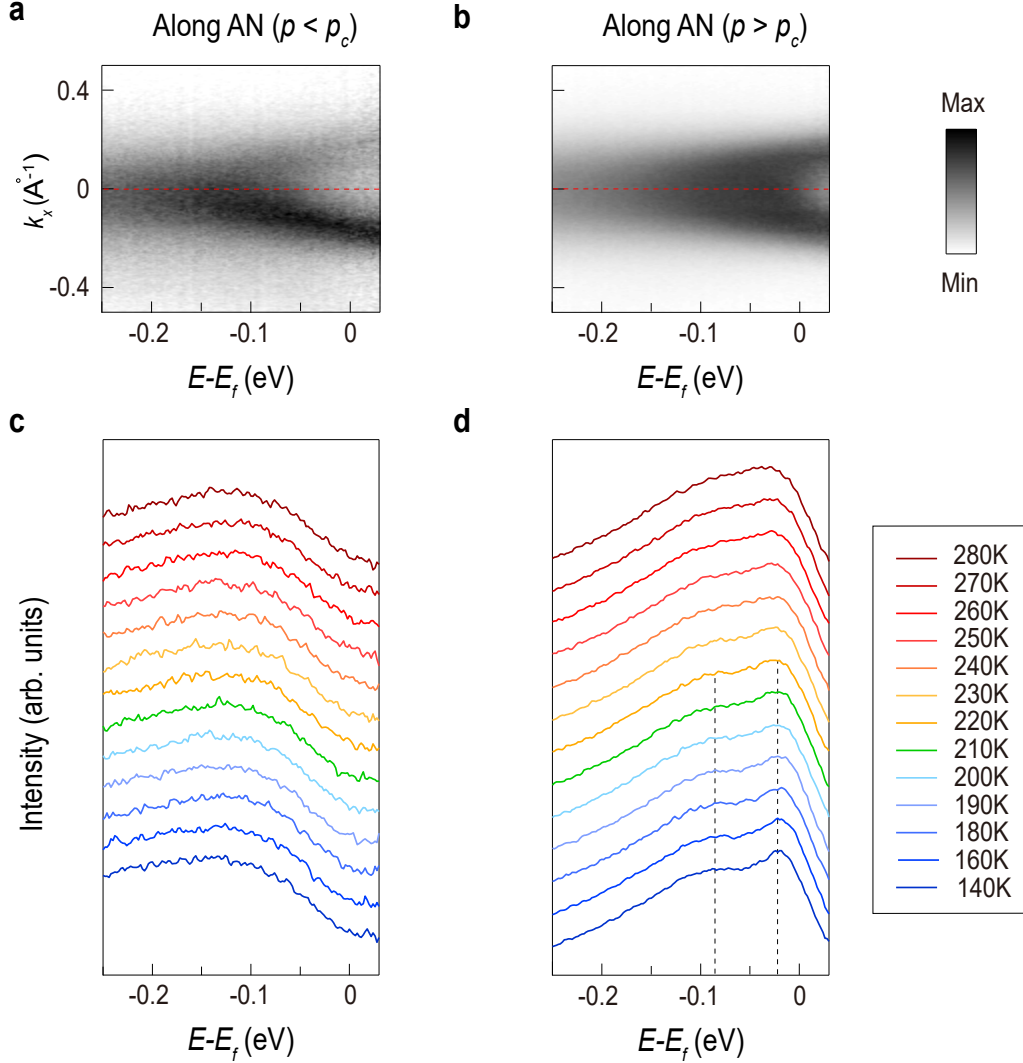

Fig. S10. **ARPES spectra along the antinodal direction for  $p < p_c$  and  $p > p_c$ .** ARPES spectra taken along the antinodal direction for (a)  $p < p_c$  ( $p=0.195$ ) and (b)  $p > p_c$  ( $p=0.205$ ) taken at  $T = 280$  K. (c,d) Temperature dependent of EDCs at the antinode (red dotted line in (a) and (b)). Dotted lines in (d) denote appearance of the coherent bilayer splitting between the bonding and anti-bonding states below  $T_{up} \sim 225$  K.

## 12. RA-SHG data from Pb-Bi2212 with $p < p_c$

We also measured RA-SHG on Pb-Bi2212 with  $T_c = 89$  K,  $T^* \sim 150$  K and  $p \sim 0.185$ , of which doping level is  $p < p_c$ . As-grown Pb-Bi2212 crystals were annealed in  $N_2$  for 48 hours at  $600^\circ\text{C}$  to control the doping level. Figure S11a shows RA-SHG patterns of the sample acquired in the  $S_{in}S_{out}$  (SS) polarization geometry at  $T \sim 295$  K and 70 K. Note that the polar data exhibits the absence of the mirror symmetry along the crystal axis even at room temperature, in contrast to the as-grown Pb-Bi2212 case in the main text. A previous report shows that the dopant oxygen atoms in Pb-Bi2212 can aggravate the distortions in the local atomic arrangement [6]. In the same way, the absence of the mirror symmetry in annealed sample may come from oxygen vacancy-induced monoclinic distortions. This monoclinic distortion is also captured in the fitting result. Our SHG data at room temperature was fitted to a bulk electric-quadrupole (EQ) contribution from  $2/m$  monoclinic crystallographic point groups as indicated by the red solid line. The blue solid line indicates a simple magnification ( $\times 1.45$ ) of the room temperature data fit result.

We tracked the temperature dependence of the SHG intensity in fine temperature steps with  $\varphi$  fixed to the maximum lobe intensity angle. We then normalized the data to the value at  $T \sim 190$  K ( $I_{SS}^{2\omega}$ ). Finally, a linear-in temperature background is subtracted from  $I_{SS}^{2\omega}$  and plotted in the figure. We can clearly see an order parameter-like sudden increase near the pseudogap temperature  $T^* \sim 150$  K.

This result is compatible with a previous RA-SHG experiment on  $\text{YBa}_2\text{Cu}_3\text{O}_y$  in two aspects. First, the room temperature data is fitted with  $2/m$  symmetry. Second, there is an order parameter-like upturn behavior at the pseudogap temperature. These results lead us to a conclusion that the observed onset behavior beyond the critical doping does not come from simple defects or impurities. Rather, it should come from a doping dependent behavior.

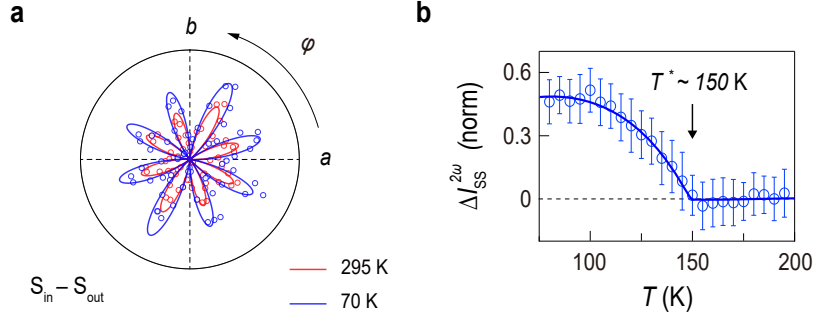

Fig. S11. **RA-SHG data from Pb-Bi2212 with  $p < p_c$ .** (a) RA-SHG polar pattern in the SS geometry at  $T = 295$  K and 70 K. Both data could be fitted to EQ induced SHG from  $2/m$  (red and blue lines). (b) Temperature dependent RA-SHG intensity in the SS geometry. Data was first normalized to the value at  $T \sim 190$  K, and then a high-temperature linear background was subtracted. The error bars represent the standard deviation in the intensity for 60 independent measurements. The blue solid line is a guide to the eyes.

---

\* Deceased

† Corresponding autor: dongjoon.song@ubc.ca

‡ Corresponding autor: changyoung@snu.ac.kr

- [1] Raab, R. E. & De Lange, O. L. *Multipole theory in electromagnetism: classical, quantum, and symmetry aspects, with applications*, vol. 128 (OUP Oxford, 2004).
- [2] Birss, R. R. *Symmetry and magnetism*, (North-Holland Pub. Co., Amsterdam., 1964.).
- [3] Kim, S. *et al.* A compact and stable incidence-plane-rotating second harmonics detector. *Review of Scientific Instruments* **92**, 043905 (2021).
- [4] Jeong, D. & Lee, J. Surface symmetry determination by a deep learning application of optical second-harmonic generation results. *Results in Physics* **40**, 105869 (2022).
- [5] Chen, S.-D. *et al.* Incoherent strange metal sharply bounded by a critical doping in bi2212. *Science* **366**, 1099–1102 (2019).
- [6] Song, D. *et al.* Visualization of dopant oxygen atoms in a  $\text{bi2sr2cacu2o8} + \delta$  superconductor. *Advanced Functional Materials* **29**, 1903843 (2019).
